# Supplementary material for: On the Effects of Smoothing Rugged Landscape by Different Toy Problems: A Case Study on UBQP
Source: arXiv:2407.19676 ancillary file (2024-07-29)
Supplement: Supplementary file 1 [file Slides--Smoothing_UBQP_landscape_with_different_toy_problems.pdf]

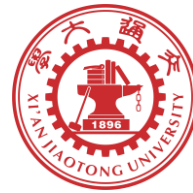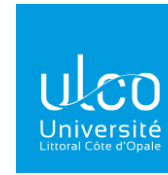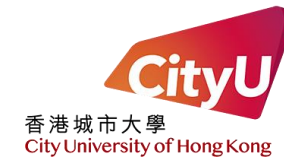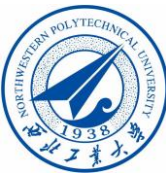

# On the Effects of Smoothing Rugged Landscape by Different Toy Problems: A Case Study on UBQP

Wei Wang<sup>1</sup>, Jialong Shi<sup>1</sup>, Jianyong Sun<sup>1</sup>,  
Arnaud Liefoghe<sup>2</sup>, Qingfu Zhang<sup>3</sup>, Ye Fan<sup>4</sup>

<sup>1</sup>Xi'an Jiaotong University, Xi'an, China

<sup>2</sup>Université du Littoral Côte d'Opale (ULCO), Calais, France

<sup>3</sup>City University of Hong Kong, Hong Kong, China

<sup>4</sup>Northwestern Polytechnical University, Xi'an, China

# Outline

- I. Introduction
- II. Research Contents
- III. Experimental Results
- IV. Conclusion

# Part 1. Introduction

*On the Effects of Smoothing Rugged Landscape by Different Toy Problems: A Case Study on UBQP (CEC2024)*

# Unconstrained Binary Quadratic Programming (UBQP)

- **Definition of UBQP**

$$\text{maximize } f(x) = x^T Q x = \sum_{i=1}^n \sum_{j=1}^n Q_{ij} x_i x_j$$

$$x \in \{0,1\}^n$$

$$Q = [Q_{ij}]: n \times n\text{-dimensional matrix}$$

**NP-Hard**

- **Fitness landscape:  $(S, V, f)$**

**Search Space  $(S)$ :** binary strings of length  $n$

**Neighborhood  $(V)$ :**  $V: S \rightarrow 2^S$ , 1-bit-flip,  $V|s| = n$

**Fitness  $(f)$ :**  $S \rightarrow R$

Landscape of UBQP is rugged

Many local optima

Hard for iterative algorithms

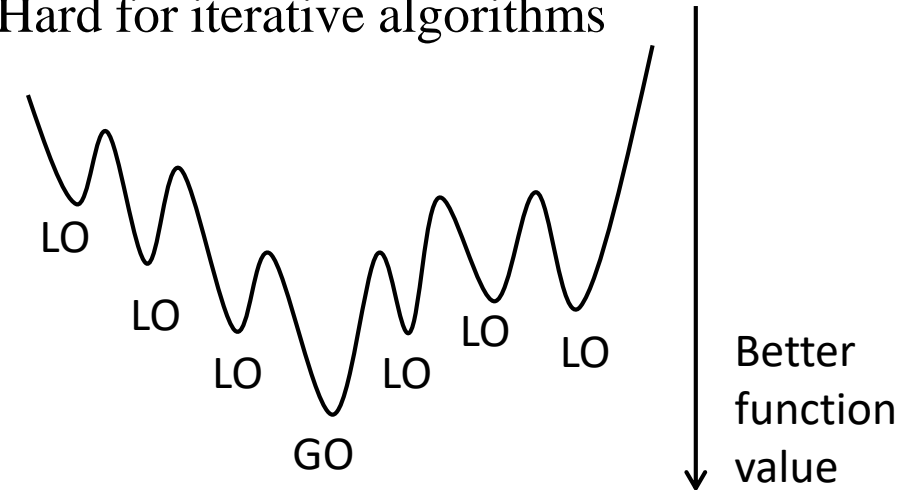

# Constructing a toy unimodal UBQP

- Given a binary strings  $x^*$  of any size
- A toy unimodal UBQP  $\hat{Q}^1$  can be constructed by

“+/-1” strategy<sup>[1]</sup>:

$$\hat{Q}_{ij}^1 = \begin{cases} 1, & \text{if } x_i^* x_j^* = 1 \\ -1, & \text{if } x_i^* x_j^* \neq 1 \end{cases}, \quad i, j \in \{1, 2, \dots, n\}$$

- Example:**

$$x^* = (0, 1, 0)$$

$$\hat{Q}^1 = \begin{bmatrix} -1 & -1 & -1 \\ -1 & 1 & -1 \\ -1 & -1 & -1 \end{bmatrix}$$

Toy UBQP:

$$\text{maximize } f(x) = x^\top \hat{Q}^1 x$$

The landscape of  $\hat{Q}^1$  seems to be like:

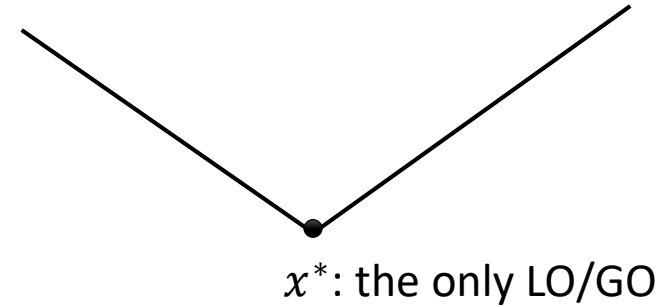

| $x$             | $f(x)$ | 1-bit-LO? | 2-bit-LO? | 3-bit-LO(GO)? |
|-----------------|--------|-----------|-----------|---------------|
| (1, 1, 1)       | -4     | no        | no        | no            |
| (1, 0, 1)       | -3     | no        | no        | no            |
| (1, 0, 0)       | -1     | no        | no        | no            |
| (1, 1, 0)       | -1     | no        | no        | no            |
| (0, 0, 1)       | -1     | no        | no        | no            |
| (0, 1, 1)       | -1     | no        | no        | no            |
| (0, 0, 0)       | 0      | no        | no        | no            |
| $x^*=(0, 1, 0)$ | 1      | YES       | YES       | YES           |

# Smoothing rugged landscape by unimodal landscape

- Homotopic convex transformation (HC transfer)
  - First proposed for TSP<sup>[2]</sup>
  - Unimodal toy TSP:
    - all cities lying on a convex hull in 2D space
- **HC transfer also can smooth UBQP<sup>[1]</sup>.**

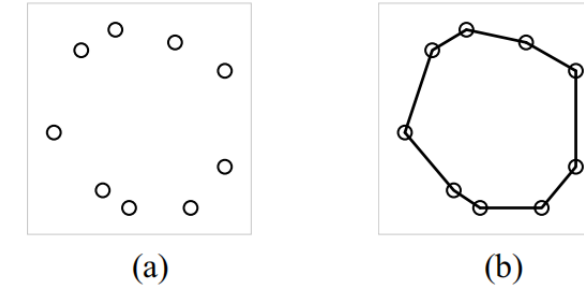

Fig. 2. Example of the (a) convex-hull TSP and the (b) corresponding global optimum.

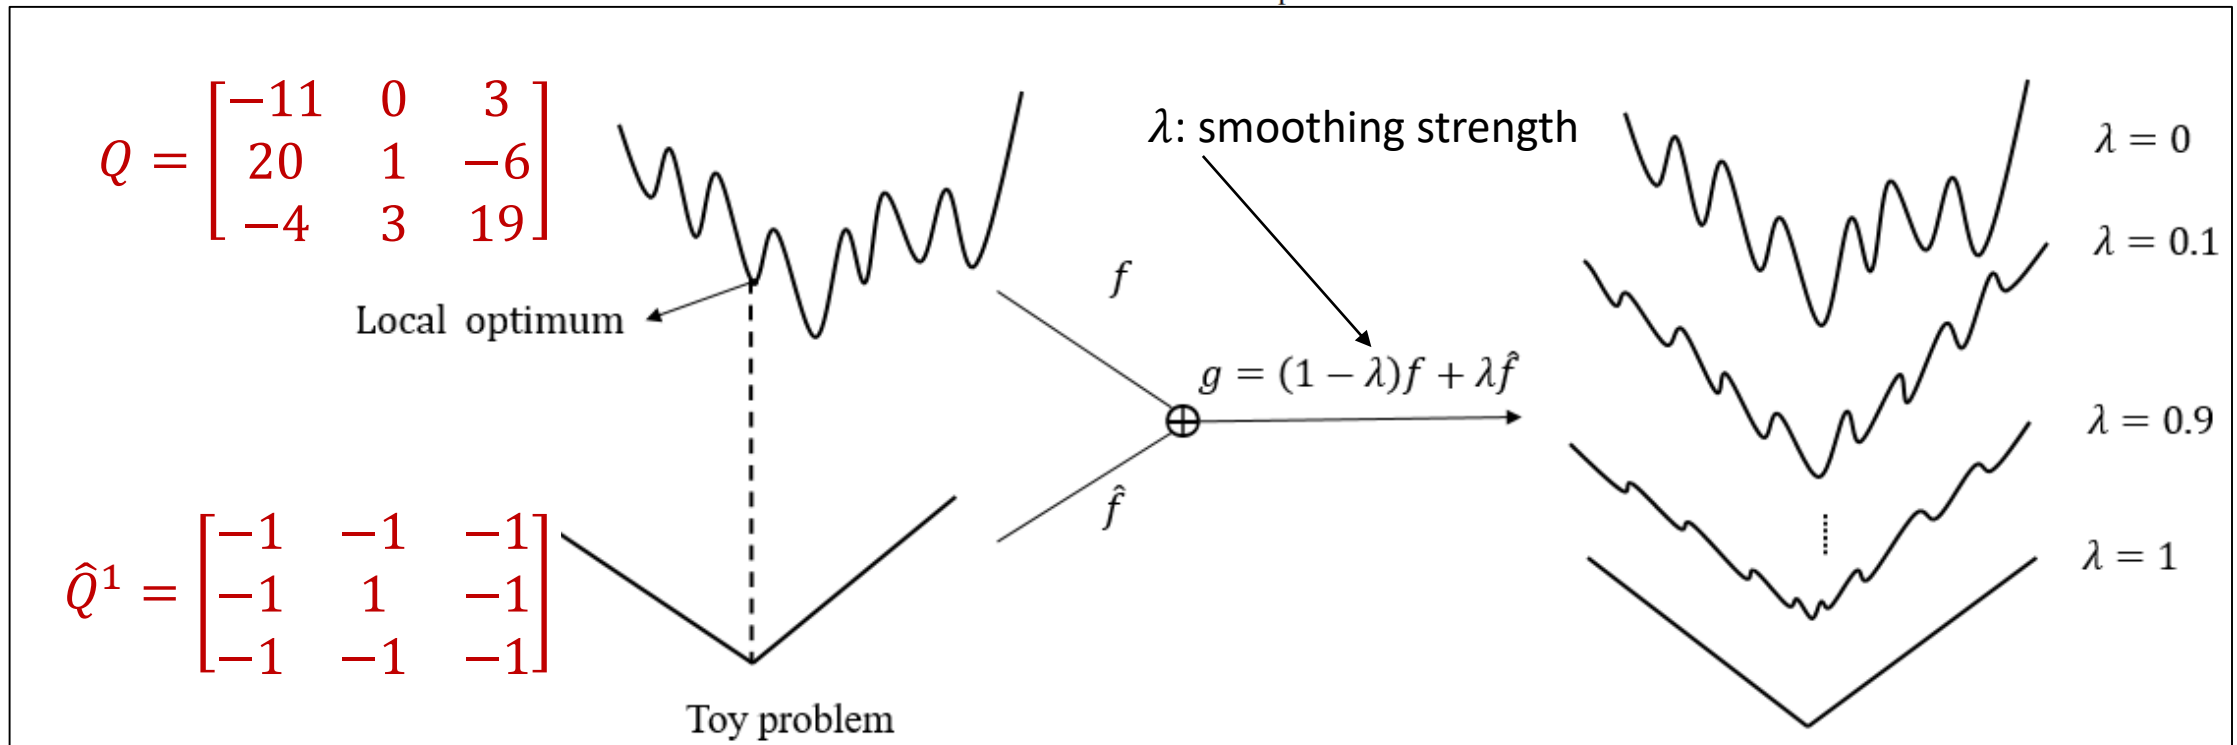

[1] W. Wang, J. Shi, J. Sun, A. Liefoghe, and Q. Zhang, "A New Parallel Cooperative Landscape Smoothing Algorithm and Its Applications on TSP and UBQP." arXiv e-prints arXiv:2401.03237, 2024.

[2] J. Shi, J. Sun, Q. Zhang and K. Ye, "Homotopic Convex Transformation: A New Landscape Smoothing Method for the Traveling Salesman Problem," in IEEE Transactions on Cybernetics, vol. 52, no. 1, pp. 495-507, 2022

# Landscape Smoothing Iterated Local Search (LSILS)

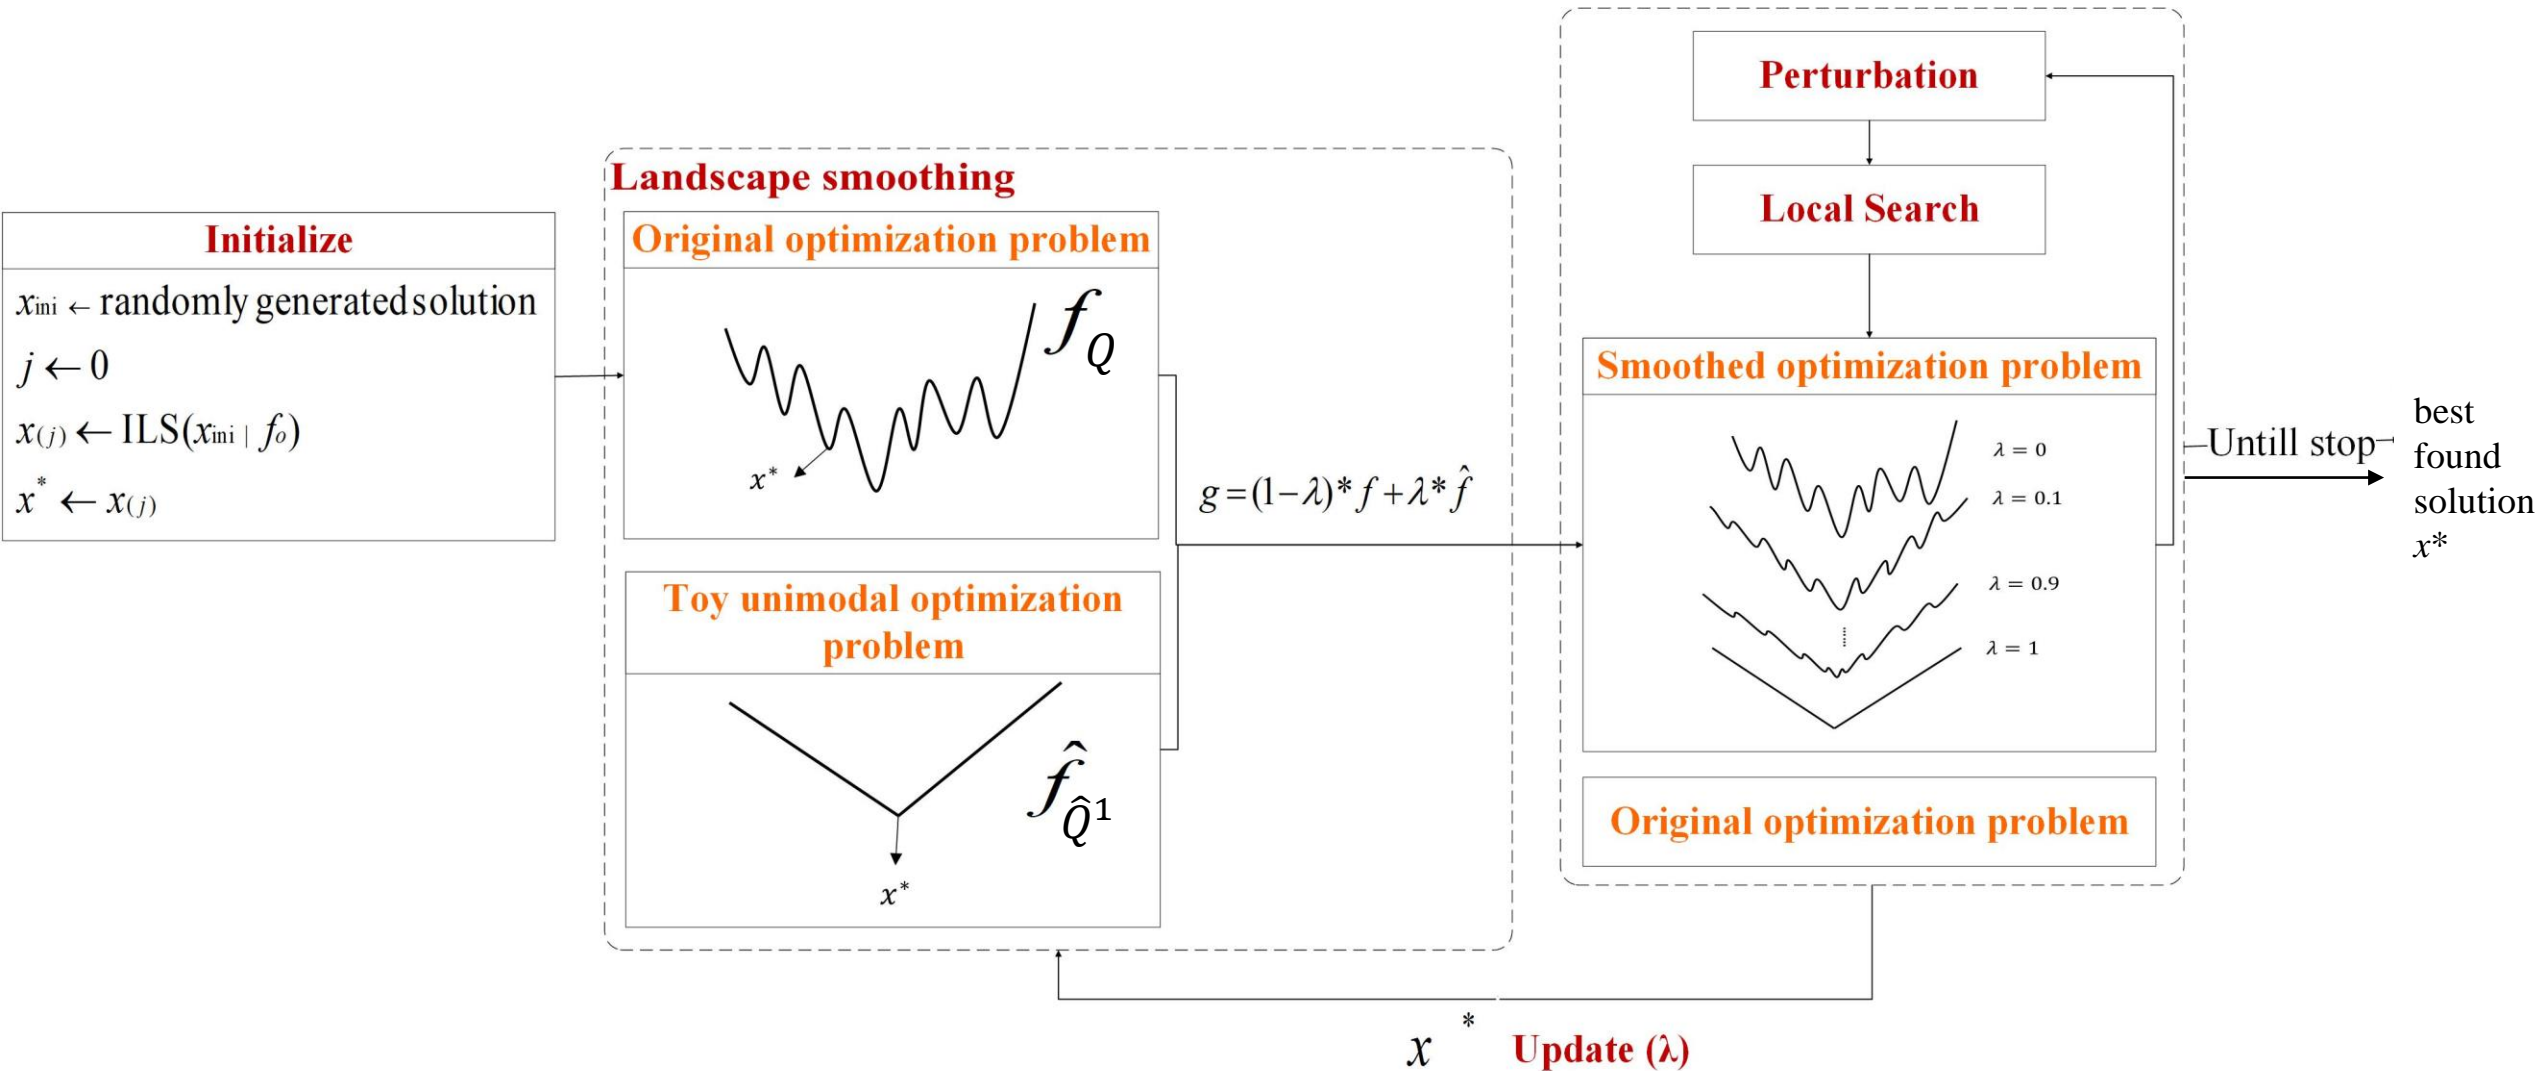

Is  $\hat{Q}^1$  the best choice for LSILS?

# Drawback of $\hat{Q}^1$ : unimodal but flat

**18-dimensional example:**

$$x^* = (1, 1, 0, 0, 1, 0, 0, 0, 0, 0, 1, 1, 1, 1, 1, 1, 1, 0),$$

$$\hat{Q}^1 = \begin{bmatrix} 1 & 1 & \cdots & 1 & -1 \\ 1 & 1 & \cdots & 1 & -1 \\ \vdots & \vdots & \ddots & \vdots & \vdots \\ 1 & 1 & \cdots & 1 & -1 \\ -1 & -1 & \cdots & -1 & -1 \end{bmatrix}$$

**Distribution of solution space of  $\hat{Q}^1$  :**

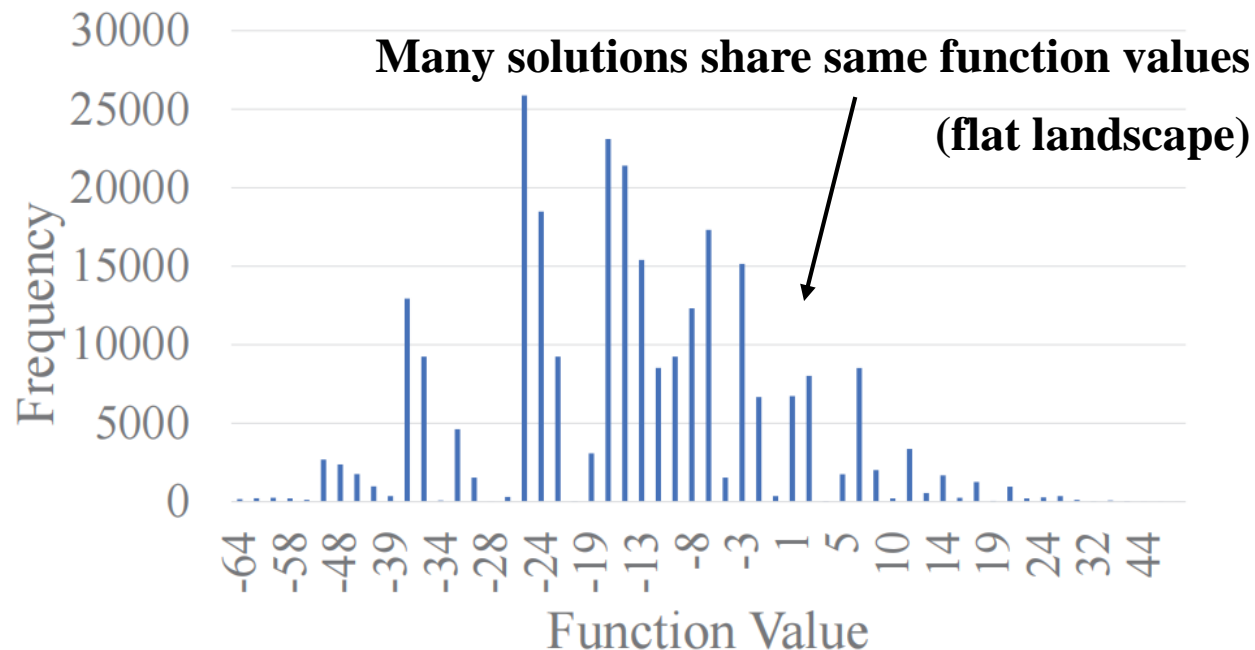

The landscape of  $\hat{Q}^1$  actually is like:

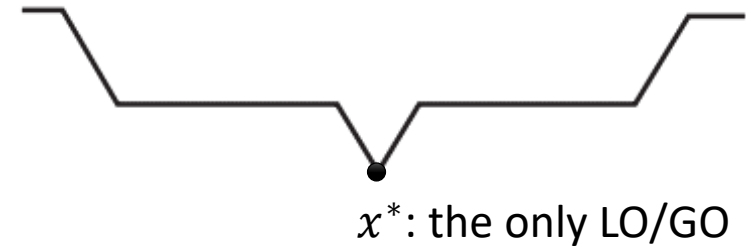

**Flatness also is challenging for iterative algorithms**

What we expect:

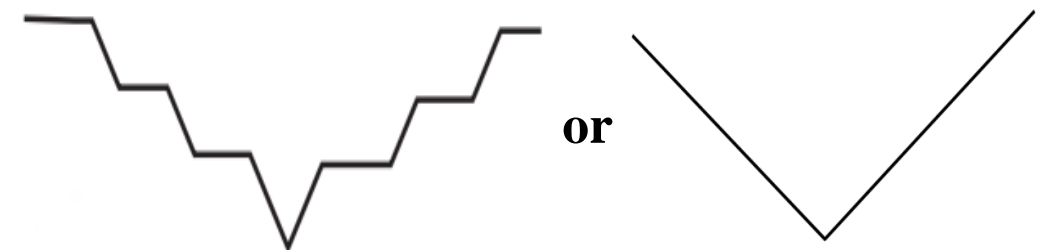

**New toy UBQP needs to be constructed**



# Part 2. Research Contents

# Toy unimodal UBQP with less flat landscape

$\hat{Q}^2$  (construct by “+/-i” strategy)

$$\hat{Q}_{ij}^2 = \begin{cases} i, & \text{if } x_i^* x_j^* = 1 \\ -i, & \text{if } x_i^* x_j^* \neq 1 \end{cases}$$

$i \in \{1, 2, \dots, n\}$  and  $j \in \{1, 2, \dots, i\}$ ,

let  $\hat{Q}_{ij}^2 = \hat{Q}_{ji}^2$

**Example:**  $x^* = (0 \ 1 \ 0 \ 1 \ 1)$

$$\hat{Q}^2 = \begin{bmatrix} -1 & -2 & -3 & -4 & -5 \\ -2 & 2 & -3 & 4 & 5 \\ -3 & -3 & -3 & -4 & -5 \\ -4 & 4 & -4 & 4 & 5 \\ -5 & 5 & -5 & 5 & 5 \end{bmatrix}$$

**Distribution of solution space of  $\hat{Q}^2$ :**

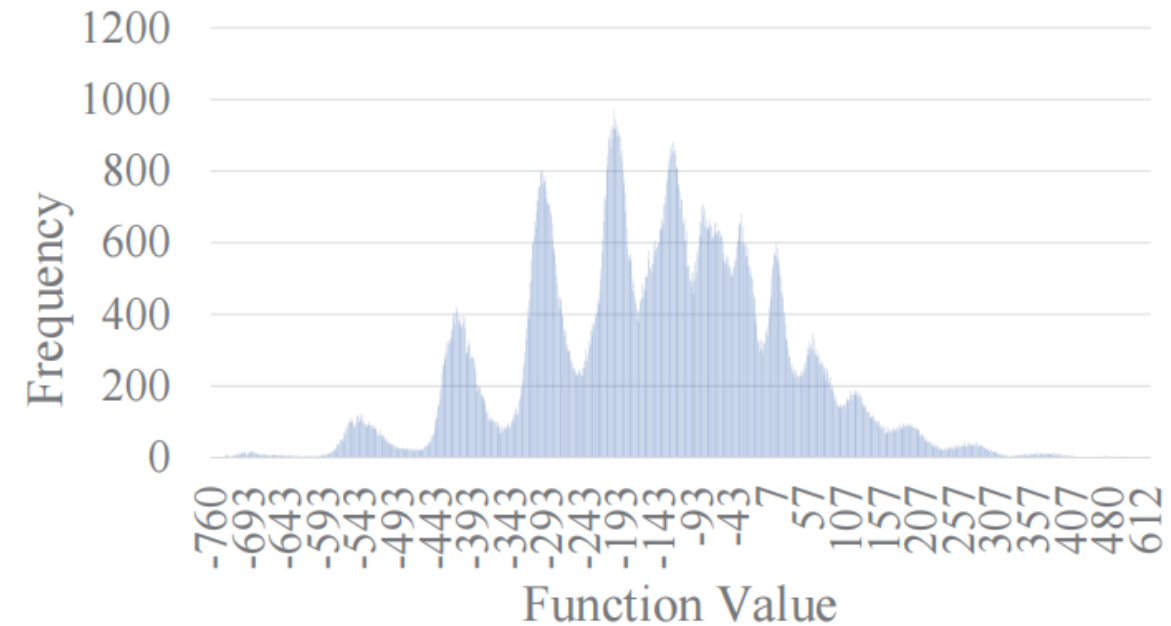

$\hat{Q}^2$  is **less flatter** than  $\hat{Q}^1$

It can be proved that  $\hat{Q}^2$  has a unimodal landscape

# Toy unimodal UBQP with less flat landscape

$\hat{Q}^3$  (construct by **randomly strategy**)

$$\hat{Q}_{ij}^3 = \begin{cases} u_{ij}^1, & \text{if } x_i^* x_j^* = 1 \\ u_{ij}^2, & \text{if } x_i^* x_j^* \neq 1 \end{cases}$$

$i \in \{1, 2, \dots, n\}$  and  $j \in \{1, 2, \dots, i\}$ ,

$u_{ij}^1$ : random integer,  $P(u_{ij}^1 = k_1) = \frac{1}{100}$ ,  $k_1 \in \{1, 2, \dots, 100\}$

$u_{ij}^2$ : random integer,  $P(u_{ij}^2 = k_2) = \frac{1}{100}$ ,  $k_2 \in \{-100, \dots, -1\}$

then let  $\hat{Q}_{ij}^3 = \hat{Q}_{ji}^3$

**Example:**  $x^* = (0 \ 1 \ 0 \ 1 \ 1)$

$$\hat{Q}^3 = \begin{bmatrix} -33 & -27 & -52 & -46 & -40 \\ -27 & 62 & -72 & 95 & 11 \\ -52 & -72 & -24 & -18 & -44 \\ -46 & 95 & -18 & 1 & 17 \\ -40 & 11 & -44 & 17 & 21 \end{bmatrix}$$

It can be proved that  $\hat{Q}^3$  has a unimodal landscape

**Distribution of solution space of  $\hat{Q}^3$  :**

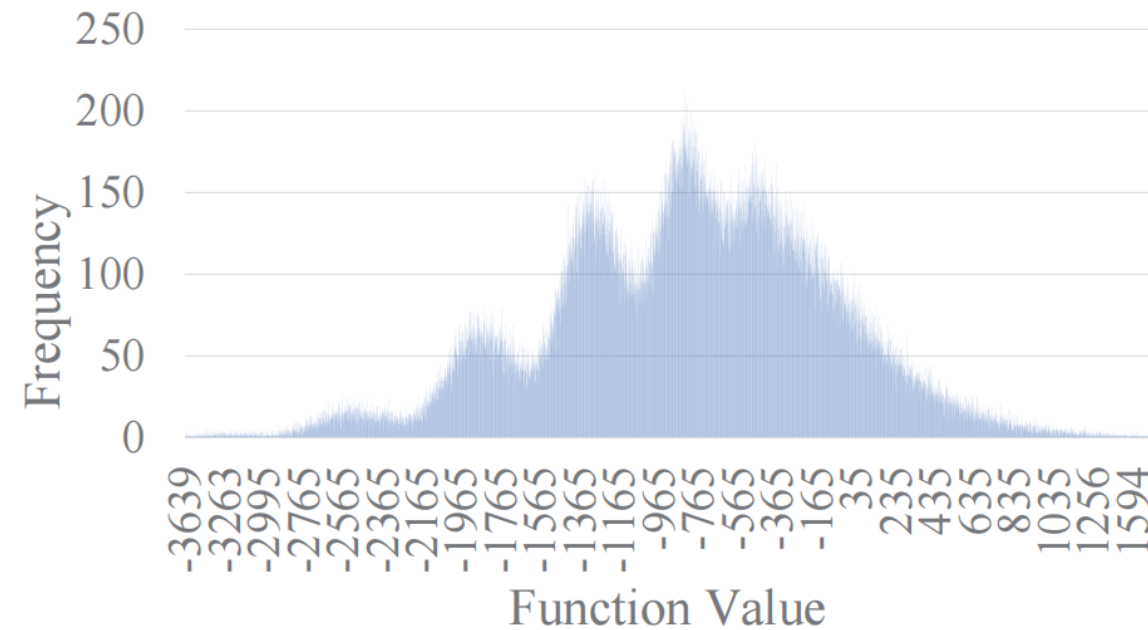

$\hat{Q}^3$  is **less flatter** than  $\hat{Q}^2$

Less flat

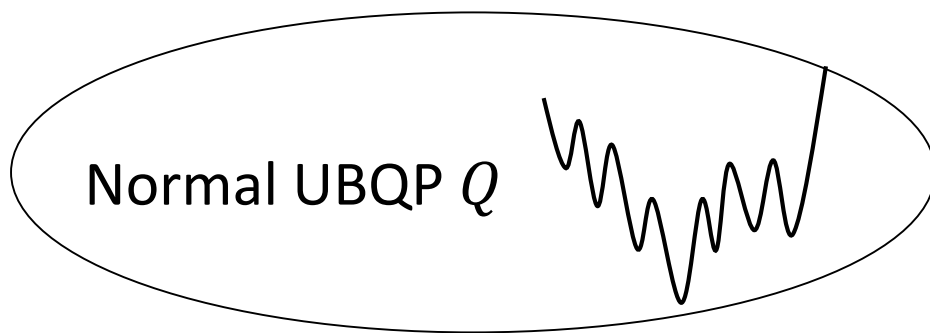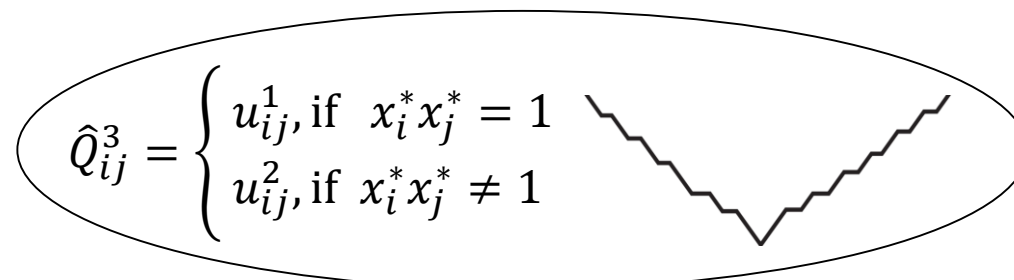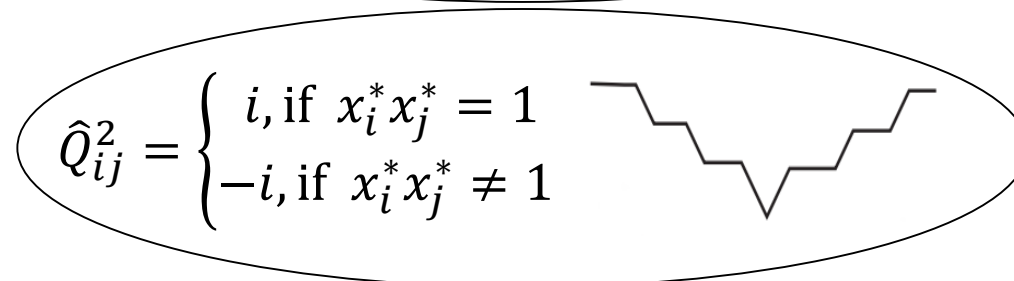

Multi-modal

Unimodal

flat

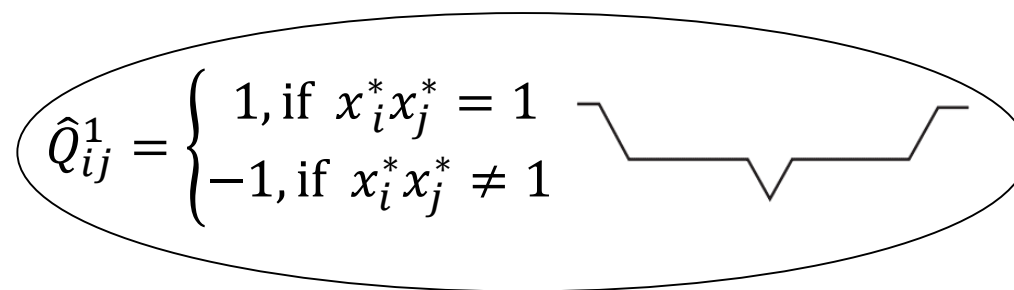

# Part 3. Experimental Results

*On the Effects of Smoothing Rugged Landscape by Different Toy Problems: A Case Study on UBQP (CEC2024)*

# Effects of smoothing

18-dimensional UBQP

$2^{18} = 262144$  solutions in solution space

$x^* = (1, 1, 0, 0, 1, 0, 0, 0, 0, 0, 1, 1, 1, 1, 1, 1, 1, 0)$

| Instance                          | Number of local optimum | 1-bit local optimum                                                                                                                                                                                                                                                                                                                             |
|-----------------------------------|-------------------------|-------------------------------------------------------------------------------------------------------------------------------------------------------------------------------------------------------------------------------------------------------------------------------------------------------------------------------------------------|
| Original randomly generated $Q$   | 5                       | $x_1 = (0, 1, 0, 0, 0, 0, 0, 1, 1, 1, 0, 1, 1, 0, 0, 0, 0, 0)$<br>$x_2 = (1, 0, 1, 1, 1, 0, 0, 0, 1, 0, 1, 1, 1, 0, 0, 0, 1, 0)$<br>$x_3 = (1, 1, 1, 0, 1, 0, 0, 1, 1, 0, 1, 1, 1, 0, 0, 0, 1, 0)$<br>$x_4 = (0, 0, 0, 1, 1, 0, 0, 1, 1, 1, 1, 1, 1, 1, 0, 0, 0, 1, 0)$<br>$x_5 = (1, 1, 1, 0, 1, 0, 0, 1, 1, 0, 0, 1, 1, 0, 1, 0, 1, 0, 1, 0)$ |
| $\hat{Q}^1$ (construct by “+/-1”) | 1                       | $x_1 = (1, 1, 0, 0, 1, 0, 0, 0, 0, 0, 0, 1, 1, 1, 1, 1, 1, 1, 0)$                                                                                                                                                                                                                                                                               |
| $\hat{Q}^2$ (construct by “+/-i”) | 1                       | $x_1 = (1, 1, 0, 0, 1, 0, 0, 0, 0, 0, 0, 1, 1, 1, 1, 1, 1, 1, 0)$                                                                                                                                                                                                                                                                               |
| $\hat{Q}^3$ (construct randomly)  | 1                       | $x_1 = (1, 1, 0, 0, 1, 0, 0, 0, 0, 0, 0, 1, 1, 1, 1, 1, 1, 1, 0)$                                                                                                                                                                                                                                                                               |

Unimodal

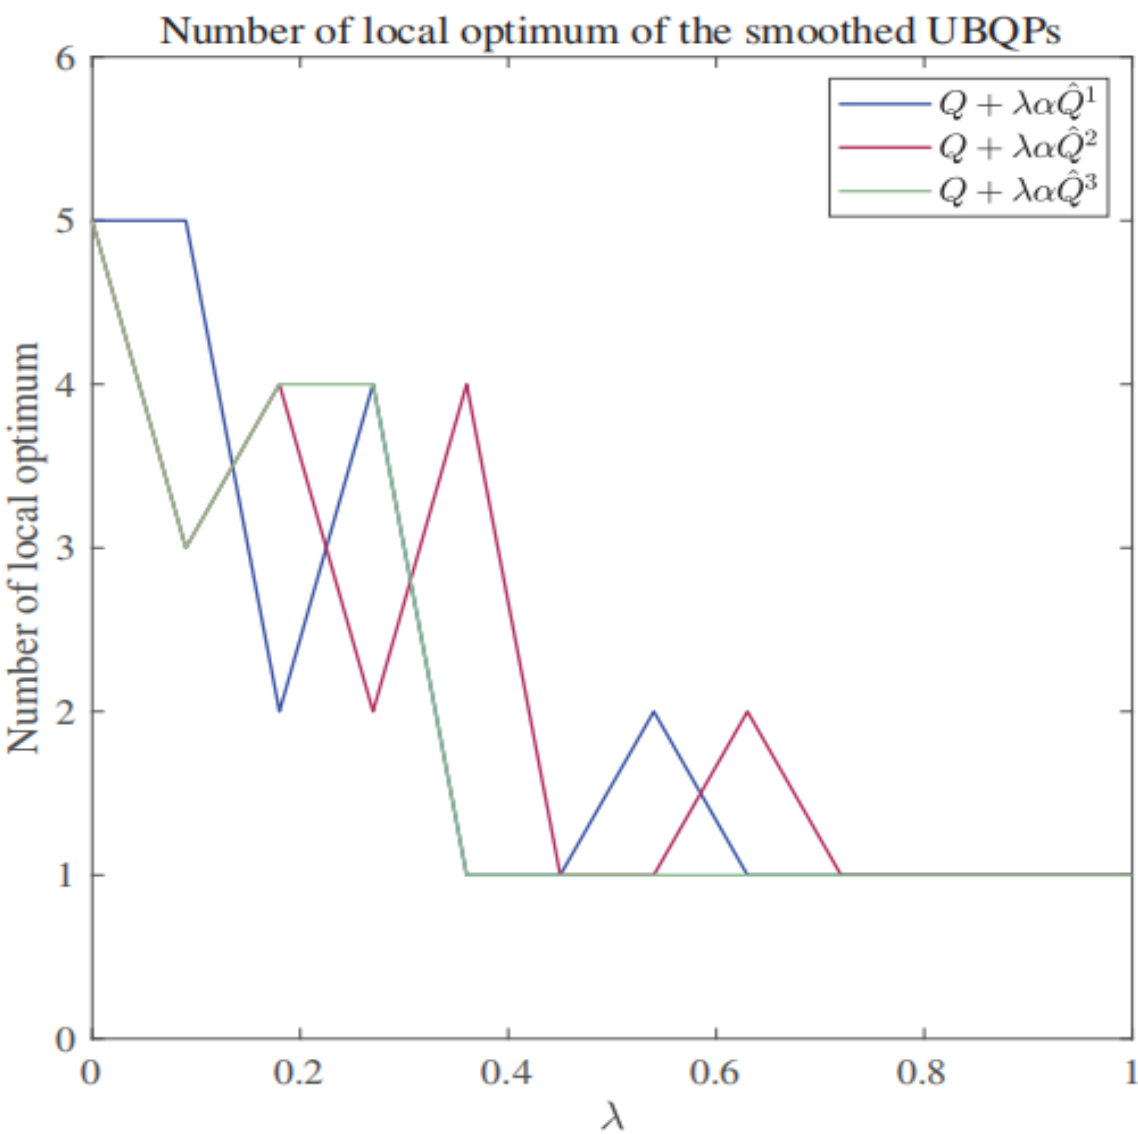

**Results:** The number of local optima is approximately negatively related to  $\lambda$ .

# Performance of LSILS with different toy unimodal UBQPs

## Experiment setting :

**Smoothing strength  $\lambda$ :** dynamically increasing ( $0 \rightarrow 0.001 \rightarrow \dots \rightarrow 0.004$ )

**Max CPU runtime:** 1000s

**Test instances:** 10 UBQPs with size 2500 from the ORLIB

## Metric:

$$excess = \frac{f(x) - f(x_{\text{opt}})}{f(x_{\text{opt}})},$$

$f(x_{\text{opt}})$ : known global optimum

# Performance of LSILS with different toy unimodal UBQPs

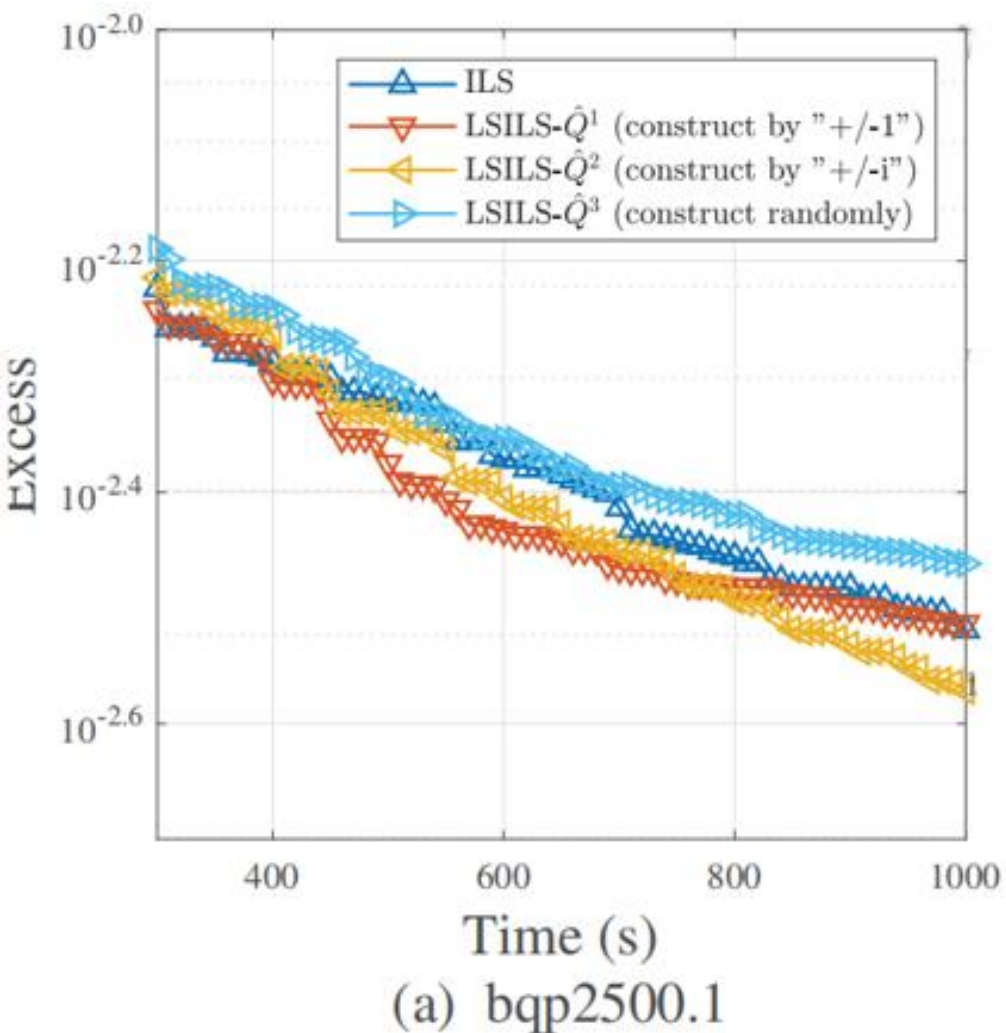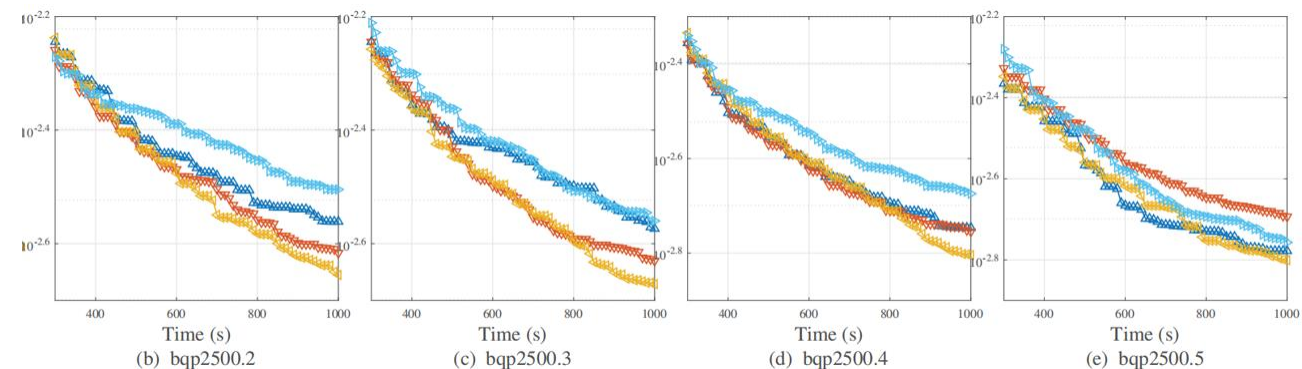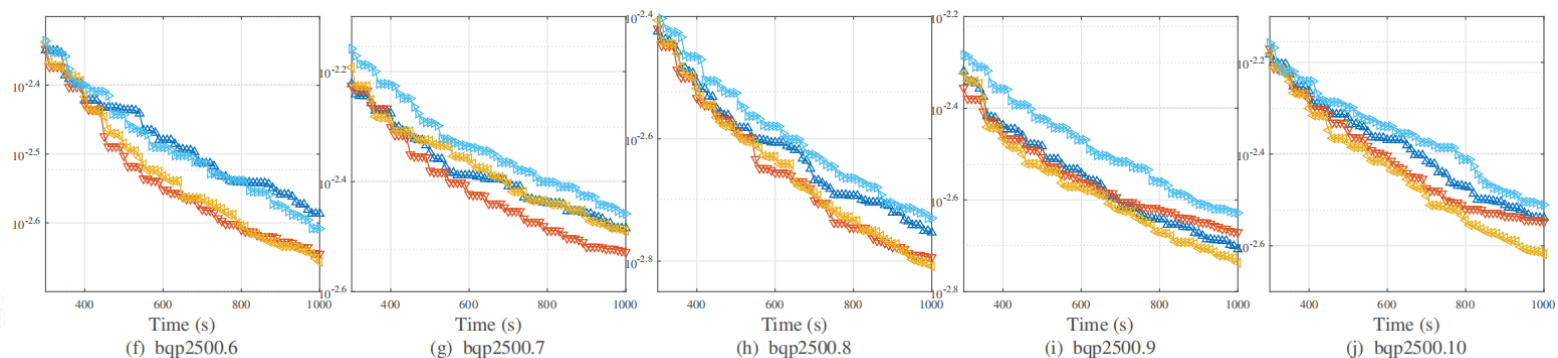

**Results:** The smoothing effect is affected by the **smoothness** and **flatness** of landscapes.



# Landscape visualization

15-dimensional UBQP ( $2^{15} = 32768$  solutions)

## 2D graph:

**Node:** solution

**Radius:** hamming distance from global optimum

**Edge:** linking 1-bit neighboring solutions

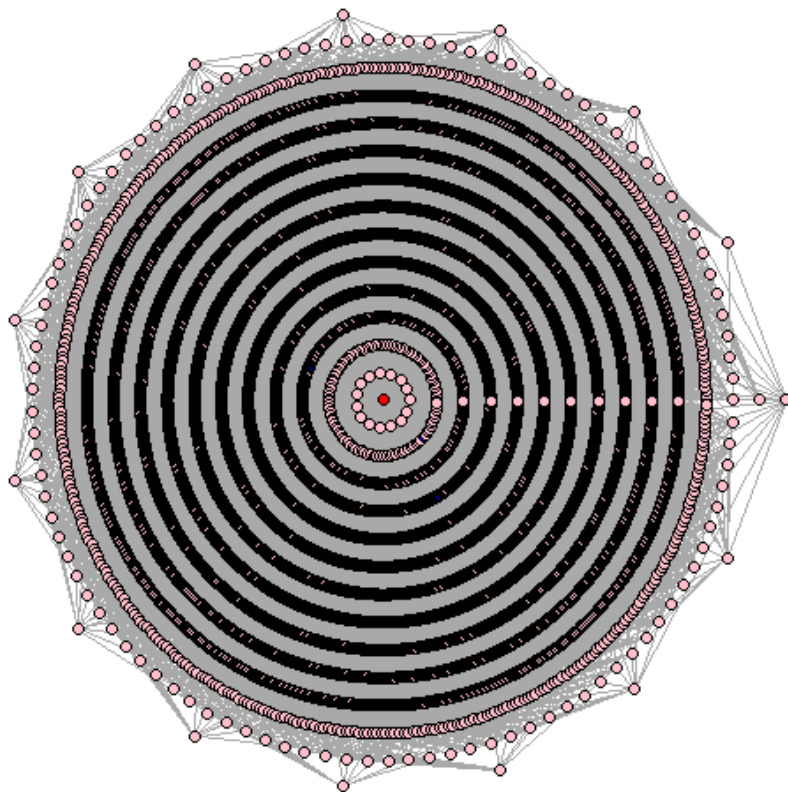

## 3D graph: function value as height

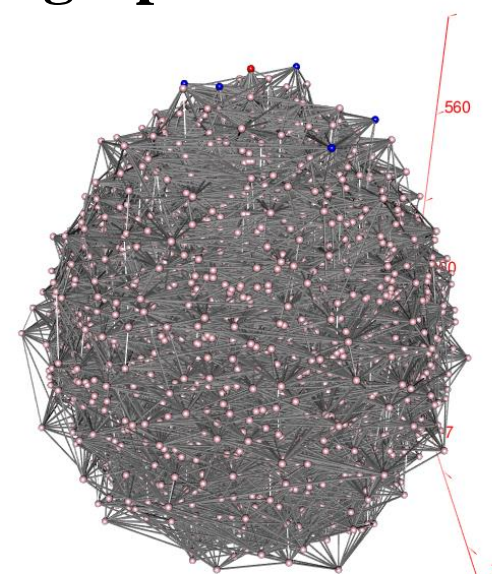

Original randomly generated  $Q$

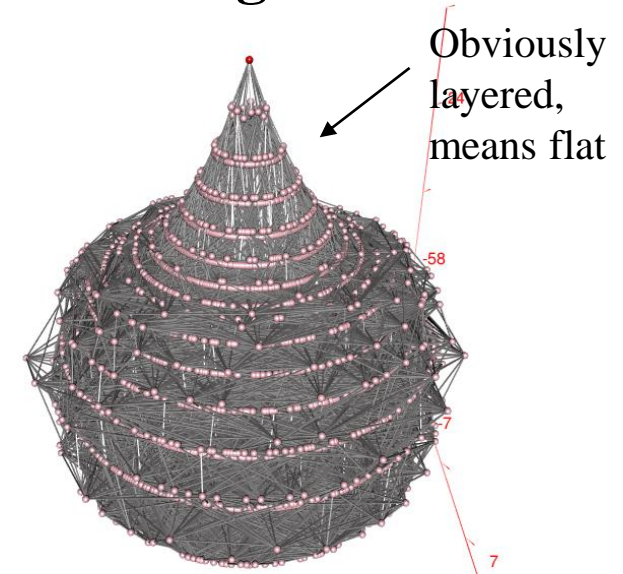

$\hat{Q}^1$  (construct by "+/-1")

Less layered,  
less flat

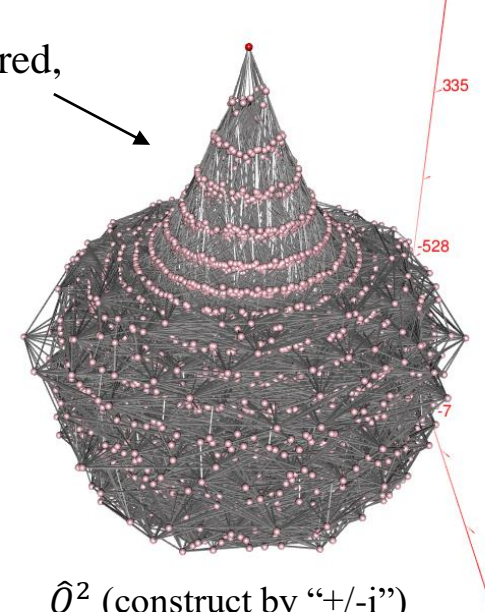

$\hat{Q}^2$  (construct by "+/-i")

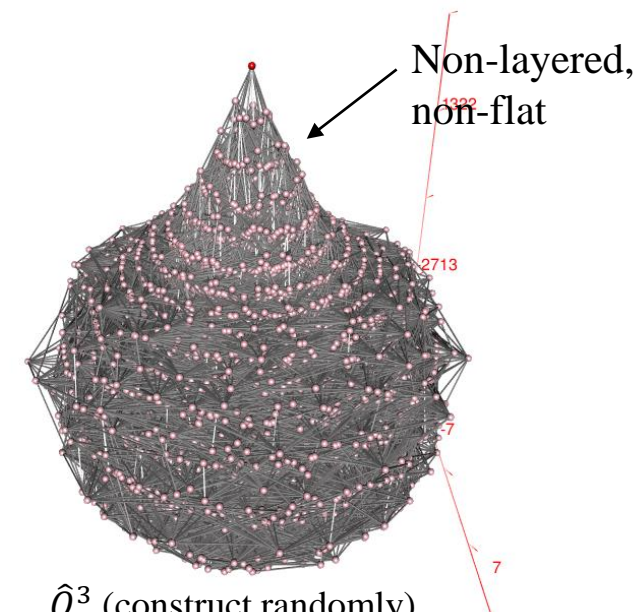

$\hat{Q}^3$  (construct randomly)

# Part 4. Conclusion

# Conclusion

- The **smoothness** and **flatness** are both important landscape characteristics.
- Different toy UBQPs have different landscape smoothing effects on the original UBQP.

## Future work

- Smoothing the landscape of Quadratic Assignment Problem (QAP).
- Landscape visualization for large-size problem

# Thanks and please refer to...

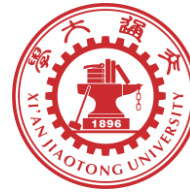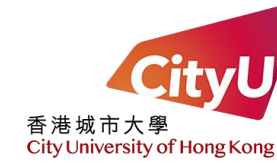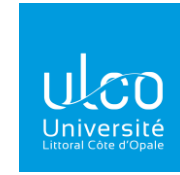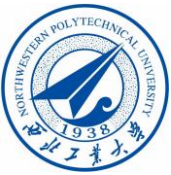

## Our papers on **combinatorial landscape smoothing**:

1. J. Shi, J. Sun, Q. Zhang and K. Ye, "Homotopic Convex Transformation: A New Landscape Smoothing Method for the Traveling Salesman Problem," in IEEE Transactions on Cybernetics, vol. 52, no. 1, pp. 495-507, 2022.  
Code: [https://github.com/JialongShi/LSILS\\_TSP\\_3opt](https://github.com/JialongShi/LSILS_TSP_3opt)
2. W. Wang, J. Shi, J. Sun, A. Liefooghe, Q. Zhang and Y. Fan, "On the Effects of Smoothing Rugged Landscape by Different Toy Problems: A Case Study on UBQP" CEC2024.
3. W. Wang, J. Shi, J. Sun, A. Liefooghe, and Q. Zhang, "A New Parallel Cooperative Landscape Smoothing Algorithm and Its Applications on TSP and UBQP." arXiv:2401.03237, 2024.
